# Supplementary material for: Prophet Inequalities with Cancellation Costs
Source: arXiv:2404.00527 source file (2026-10-12)
Supplement: Supplementary file 1 [file appendix-bounded-case.tex]

\section{The bounded random variable case}
\label{apx:bounded}
If the random variable $X_{\max}$ were to bounded within a multiplicative range of $(1+f)$, i.e., there is  $\alpha$ such that $\alpha \leq X_{\max} < (1+f)\alpha$, then there would be no profit in buying back. What is the best competitive ratio we can obtain in this case? In this section, we prove that it is $\frac{1+f}{1+2f}$, and that it can be obtained with several different threshold based algorithms.

We start with the following important lemma.

\begin{lemma} 
Suppose $X_i < (1+f)T$ for all $i$. Then, 
$$\sum_{i=1}^{n} \frac{\EX[(X_i-T)_+]}{1-\frac{\EX[(\max_{j =i}^n X_j-T)_+]}{fT}} \geq \frac{\EX[(X_{\max} - T)_+]}{1-\frac{\EX[(X_{\max} - T)_+]}{fT}}.$$
\end{lemma}
\begin{proof}
It suffices to prove the statement for $n = 2$, since the statement will then follow from a straightforward induction. Define $$Y_i = 1 - \frac{(X_i-T)_+}{fT},$$ and note that $0 \leq Y_i \leq 1$. The inequality we wish to prove is simply:
\begin{align*}
&& \frac{fT-fT\EX[Y_1]}{\EX[\min \{Y_1, Y_2\}]} +\frac{fT-fT\EX[Y_2]}{\EX[Y_2]} &\geq \frac{fT-fT\EX[\min \{Y_1, Y_2\}]}{\EX[\min \{Y_1, Y_2\}]} \\
&\Leftrightarrow& \frac{1-\EX[Y_1]}{\EX[\min \{Y_1, Y_2\}]} +\frac{1-\EX[Y_2]}{\EX[Y_2]} &\geq \frac{1-\EX[\min \{Y_1, Y_2\}]}{\EX[\min \{Y_1, Y_2\}]} \\
&\Leftrightarrow& \frac{1-\EX[Y_1]}{\EX[\min \{Y_1, Y_2\}]} +\frac{1}{\EX[Y_2]} &\geq\frac{1}{\EX[\min \{Y_1, Y_2\}]} \\
&\Leftrightarrow& \frac{-\EX[Y_1]}{\EX[\min \{Y_1, Y_2\}]} +\frac{1}{\EX[Y_2]} &\geq 0 \\
&\Leftrightarrow& \EX[\min \{Y_1, Y_2\}] &\geq \EX[Y_1]\EX[Y_2]\\
\end{align*}
But $0 \leq Y_i \leq 1$, so it follows that $$\min \{Y_1, Y_2\} \geq Y_1Y_2,$$ as needed.
\end{proof}

Our main theorem provides a number of different thresholds which work to achieve a competitive ratio of $\frac{1+f}{1+2f}$:

\begin{theorem}
Suppose $\Pr[X_{\max} < T] = x$, and that there exists $\alpha$ such that $\alpha \leq X_{\max} < (1+f)\alpha$.
Then the algorithm with $T$ as a threshold (and no buyback) achieves an expected value of at least
$$ (1-x)T + x\frac{\EX[(X_{\max} - T)_+]}{1-\frac{\EX[(X_{\max} - T)_+]}{fT}}$$
and by setting $T = \max{\left(\frac{\EX[X_{\max}](1+f)}{1+2f}, \alpha\right)}$, or by setting $x = \frac{f^2}{(1+f)(1+2f)}$, or by letting $T = \max(T^*, \alpha)$ where $T^*$ satisfies the equation $T^* = \frac{\EX[(X_{\max} - T^*)_+]}{1-\frac{\EX[(X_{\max} - T^*)_+]}{fT^*}}$ (or in other words, $\EX[(X_{\max} - T^*)_+] = \frac{f}{1+f}T^*$), we obtain a  competitive ratio of
$$\frac{1+f}{1+2f}.$$
\end{theorem}

\begin{proof}
For our algorithm, we can write:
\begin{eqnarray*}
 \EX[ALG] & = & (1-x) T + \sum_{i=1}^{n} \EX[(X_i-T)_+] \cdot \Pr[X_1,\ldots,X_{i-1} < T]. 
\end{eqnarray*}
This holds, because we get $T$ as a baseline if there is any variable above $T$, and in addition, we get $X_i - T$ if $X_i$ is the first variable above $T$. 
By the independence of $X_1,\ldots,X_n$, we can further derive:
\begin{eqnarray*}
 \EX[ALG] &= & (1-x) T + \sum_{i=1}^{n} \EX[(X_i-T)_+] \cdot \frac{\Pr[X_{\max} < T]}{\Pr[X_i,\ldots,X_n < T]} \\
& = & (1-x) T + x \sum_{i=1}^{n} \frac{\EX[(X_i-T)_+]}{\Pr[X_i,\ldots,X_n < T]} \\
& \geq & (1-x) T + x\sum_{i=1}^{n} \frac{\EX[(X_i-T)_+]}{1-\Pr[\max_{j =i}^n X_j > T]}.
\end{eqnarray*}
Note that if we assume $T\geq \alpha$, then
$$fT \cdot \indic(\max_{j =i}^n X_j > T) \geq(\max_{j =i}^n X_j-T)_+.$$
It follows that  
$$ \Pr[\max_{j =i}^n X_j > T] \geq \frac{\EX[(\max_{j =i}^n X_j-T)_+]}{fT}.$$
Hence, we may continue to analyze the sum from above as follows:
\begin{eqnarray*}
\sum_{i=1}^{n} \frac{\EX[(X_i-T)_+]}{1-\Pr[\max_{j =i}^n X_j > T]} & \geq & \sum_{i=1}^{n} \frac{\EX[(X_i-T)_+
]}{1-\frac{\EX[(\max_{j =i}^n X_j-T)_+]}{fT}} \\
& \geq &\frac{\EX[(X_{\max} - T)_+]}{1-\frac{\EX[(X_{\max} - T)_+]}{fT}}.
\end{eqnarray*}
where the last bound follows from the lemma. The bound on the performance of the algorithm follows. To derive a competitive ratio for the algorithm, let us assume without loss of generality that $\EX[X_{\max}] = 1$, and note that:
\begin{eqnarray*}
&&(1-x)T + x\frac{\EX[(X_{\max} - T)_+]}{1-\frac{\EX[(X_{\max} - T)_+]}{fT}}\\
&\geq & (1-x)T + x\frac{fT(1-T)}{(1+f)T-1}.
\end{eqnarray*}
Setting $T = \frac{1+f}{1+2f}$, we obtain a competitive ratio of $\frac{1+f}{1+2f}$. Alternatively, note that $$\frac{fT(1-T)}{(1+f)T-1} \geq \frac{1+f}{1+2f} - \frac{f^2+3f+1}{f^2}\left(T-\frac{1+f}{1+2f}\right) \text{ for } T \geq \frac{1}{1+f}.$$
(This follows from the convexity of $\frac{fT(1-T)}{(1+f)T-1}$ at $T = \frac{1+f}{1+2f}$). So choosing $$x = \frac{f^2}{(1+f)(1+2f)}$$ also guarantees a competitive ratio of $\frac{1+f}{1+2f}$. Finally, setting $T = \frac{\EX[(X_{\max} - T)_+]}{1-\frac{\EX[(X_{\max} - T)_+]}{fT}}$, we are guaranteed a competitive ratio of $T$. This $T$ must be at least $\frac{fT(1-T)}{(1+f)T-1}$ (since $\frac{\EX[(X_{\max} - T)_+]}{1-\frac{\EX[(X_{\max} - T)_+]}{fT}}\geq \frac{fT(1-T)}{(1+f)T-1}$), so $T \geq \frac{1+f}{1+2f}$, as required.\end{proof}

% \end{document}
