# Supplementary material for: Prophet Inequalities with Cancellation Costs
Source: arXiv:2404.00527 source file (2026-10-12)
Supplement: Supplementary file 2 [file appendix-threshold-algorithm.tex]

\section{Analysis of threshold greedy for large buyback factors}
\label{apx:thresholdgreedy}
In the following, we aim to obtain a constant improvement over $1/2$ for any fixed buyback factor using the simple threshold-greedy algorithm. We consider the algorithm in 3 different cases.

\subsection{Case 1: not much value above the median}

Let $T = \med(X_{\max})$ and $\EX[(X_{\max} - T)_+] = \beta \cdot \EX[X_{\max}]$.
If $\beta$ is relatively small, then we prove that the basic algorithm without any buybacks already achieves an improvement over $1/2$.

\begin{lemma}
\label{lemma:case1}
Let $T = \med(X_{\max})$, $\EX[(T - X_{\max})_+] = \alpha T$ and $\EX[(X_{\max} - T)_+] = \beta \cdot \EX[X_{\max}]$ for some $\alpha, \beta \geq 0$. Then the algorithm with threshold $T$ for $\alpha \geq \frac{1-2\beta}{8-9\beta}$, or $T' = (1-3\alpha)T$ for $\alpha < \frac{1-2\beta}{8-9\beta}$, and no buybacks, achieves 
$$ \EX[ALG] \geq \frac{4-\beta}{7} \cdot \EX[X_{\max}].$$
\end{lemma}

\begin{proof}
We can assume that $\beta < \frac{1}{2}$, otherwise the statement of the lemma follows from the classical prophet inequality. Given the definitions of $\alpha, \beta$, we can write
$$ \EX[X_{\max}] = \EX[T + (X_{\max} - T)_+ + (X_{\max} - T)_-] = T + \beta \EX[X_{\max}] - \alpha T.$$
From here,
$$ \EX[X_{\max}] = \frac{1-\alpha}{1-\beta} \, T.$$

We consider first $\alpha \geq \frac{1-2\beta}{8-9\beta}$ and the algorithm with threshold $T$. In this case, the classical bound already provides an improvement over $1/2$:
\begin{eqnarray*}
\EX[ALG] & \geq & T \cdot \Pr[X_{\max} \geq T] + \EX[(X_{\max} - T)_+] \cdot \Pr[X_{\max} < T] \\
 & = & \frac12 T + \frac12 \beta \cdot \EX[X_{\max}] \\\
 & = & \frac{1-\beta}{2(1-\alpha)} \cdot \EX[X_{\max}] + \frac12 \beta \cdot \EX[X_{\max}] \\
 & = & \frac{1 - \alpha \beta}{2(1 - \alpha)} \cdot \EX[X_{\max}]
\end{eqnarray*}
For $\beta < 1$, this is an increasing function of $\alpha$, and hence it is minimized for this case at $\alpha = \frac{1-2\beta}{8-9\beta}$:
$$ \EX[ALG] \geq \frac{4 - \beta}{7} \cdot \EX[X_{\max}].$$

The second case is that $\alpha \leq \frac{1-2\beta}{8-9\beta}$ (intuitively, $X_{\max}$ is concentrated around $T$), in which case we choose $T' = (1-3\alpha) T$ as the threshold. In this case, the classical bound again gives
\begin{eqnarray*}
\EX[ALG] & \geq & T' \cdot \Pr[X_{\max} \geq T'] + \EX[(X_{\max} - T')_+] \cdot \Pr[X_{\max} < T'] \\
& \geq & T' \cdot (1 - \Pr[X_{\max} < T']) + \EX[X_{\max} - T'] \cdot \Pr[X_{\max} < T'].
\end{eqnarray*}
Let's compare $T'$ and $\EX[X_{\max} - T']$: We have $T'= (1-3\alpha) T$, and $\EX[X_{\max}]  = \frac{1-\alpha}{1-\beta} T$. Hence,
$$ \frac{T'}{\EX[X_{\max}]}  = \frac{(1-\beta)(1-3\alpha)}{1-\alpha} $$
which is a decreasing function of $\alpha$. In this case, it's minimized at $\alpha=\frac{1-2\beta}{8-9\beta}$, which gives, after some simplification, that $\frac{T'}{\EX[X_{\max}]} \geq \frac{1}{7} (5-3\beta)$. We also assume $\beta < \frac{1}{2}$, which implies
$$ \frac{T'}{\EX[X_{\max}]} > \frac{1}{2}.$$
Hence, $T'$ is larger than $\EX[X_{\max} - T']$, and the expression $T' \cdot (1 - \Pr[X_{\max} < T']) + \EX[X_{\max} - T'] \cdot \Pr[X_{\max} < T']$ is minimized when $\Pr[X_{\max} < T']$ is as large as possible. Recall that $\Pr[X_{\max} < T'] = \Pr[X_{\max} < (1-3\alpha) T] = \Pr[T - X_{\max} > 3\alpha T]$. Consider the random variable $(T-X_{\max})_+$. Its expectation is $\alpha T$, and hence by Markov's inequality, $\Pr[T-X_{\max} > 3\alpha T]  < 1/3$. We conclude,
\begin{eqnarray*}
\EX[ALG] & \geq & \frac23 T' + \frac13 \EX[X_{\max} - T'] = \frac13 T' + \frac13 \EX[X_{\max}] \\
& = & \frac{(1-\beta)(1-3\alpha)}{3 (1-\alpha)} \EX[X_{\max}] + \frac13 \EX[X_{\max}].
\end{eqnarray*}
Again, this is a decreasing function of $\alpha$, minimized at $\alpha=\frac{1-2\beta}{8-9\beta}$, and we obtain
\begin{eqnarray*}
\EX[ALG] & \geq & \frac{4 - \beta}{7} \cdot \EX[X_{\max}].
\end{eqnarray*}
\end{proof}

\subsection{Case 2: some value above the median but not enough for buyback}

Here we deal with a case where $\EX[(X_{\max} - T)_+]$ is rather large, but $ \EX[(X_{\max} - (1+f) T)_+]$ is not; i.e., we still do not have enough incentive to perform any buybacks.
In this case, we gain due to certain slack in the classical proof of the prophet inequality.

\begin{lemma}
\label{lemma:case2}
Suppose $T = \med(X_{\max})$, $\EX[(X_{\max} - T)_+] = \beta \cdot \EX[X_{\max}]$ and $\EX[(X_{\max} - (1+f)T)_+] = \gamma \cdot \EX[X_{\max}]$.
Then the algorithm with $T$ as a threshold (and no buyback) achieves
$$ \EX[ALG] \geq \left( \frac{1}{2} + \frac{(\beta - \gamma)^2}{8f (1-\beta)}\right) \ \EX[X_{\max}].$$
\end{lemma}

\begin{proof}
First we observe two bounds on $\EX[X_{\max}]$:
$$ \EX[X_{\max}] \leq T + \EX[(X_{\max} - T)_+] ,$$
$$ \EX[X_{\max}] \geq \Pr[X_{\max} \geq T] \cdot \EX[X_{\max} \mid X_{\max} \geq T]
%= \Pr[X_{\max} \geq T] \cdot \EX[T + (X_{\max} - T) \mid X_{\max} \geq T] 
 = T \cdot \Pr[X_{\max} \geq T] + \EX[(X_{\max} - T)_+] $$
$$ = \frac12 T + \beta \cdot \EX[X_{\max}], \mbox{      i.e.      }
\EX[X_{\max}] \geq \frac{T}{2(1-\beta)}.$$

For our algorithm, we can write the following lower bound:
\begin{eqnarray*}
 \EX[ALG] & \geq & T \cdot \Pr[X_{\max} \geq T] + \sum_{i=1}^{n} \EX[X_i-T] \cdot \Pr[X_1,\ldots,X_{i-1} < T, X_i \geq T] \\
 & = & \frac12 T + \sum_{i=1}^{n} \EX[(X_i-T)_+] \cdot \Pr[X_1,\ldots,X_{i-1} < T]. 
\end{eqnarray*}
This holds, because we get $T$ as a baseline if there is any variable above $T$, and in addition, we get $X_i - T$ if $X_i$ is the first variable above $T$. 
By the independence of $X_1,\ldots,X_n$, we can further derive:
\begin{eqnarray*}
 \EX[ALG] & \geq & \frac12 T + \sum_{i=1}^{n} \EX[(X_i-T)_+] \cdot \frac{\Pr[X_{\max} < T]}{\Pr[X_i,\ldots,X_n < T]} \\
& = & \frac12 T + \frac12 \sum_{i=1}^{n} \frac{\EX[(X_i-T)_+]}{\prod_{j=i}^{n} (1 - \Pr[X_j \geq T])} \\
& \geq & \frac12 T + \frac12 \sum_{i=1}^{n} \EX[(X_i-T)_+] \cdot \prod_{j=i}^{n} (1+\Pr[X_j \geq T]) \\
& \geq & \frac12 T + \frac12 \sum_{i=1}^{n} \EX[(X_i-T)_+] \cdot (1 + \sum_{j=i}^{n} \Pr[X_j \geq T]) \\
& \geq & \frac12 \EX[X_{\max}] + \frac12 \sum_{i=1}^{n} \EX[(X_i-T)_+] \sum_{j=i}^{n} \Pr[X_j \geq T].
 \end{eqnarray*}
Note that this is like the usual prophet inequality bound (with the threshold being the median of $X_{\max}$), but we have an additional term at the end. Of course, in general the prophet inequality with a factor of $\frac12$ is tight, so this additional term could be very close to $0$.
In our case, however, we can derive an additional gain.

Note that:
$$fT \cdot \indic(X_j \geq T) \geq (X_j-T)_+ - (X_j - (1+f)T)_+.$$
Let us denote $\EX[(X_j-T)_+] = \beta_j$ and $\EX[(X_j-(1+f)T)_+] = \gamma_j$. From the inequality above, 
$$ \Pr[X_j \geq T] \geq \frac{\beta_j - \gamma_j}{fT}.$$
Now consider the expression
$$ \frac12 \sum_{i=1}^{n} \EX[(X_i-T)_+] \sum_{j=i}^{n} \Pr[X_j \geq T] \geq 
\frac{1}{2fT} \sum_{i=1}^{n} \beta_i \sum_{j=i}^{n} (\beta_j - \gamma_j).
$$
We can symmetrize this expression by replacing $\beta_i$ with $\beta_i - \gamma_i$, and obtain
$$ \frac12 \sum_{i=1}^{n} \EX[(X_i-T)_+] \sum_{j=i}^{n} \Pr[X_j \geq T] \geq 
\frac{1}{2fT} \sum_{i=1}^{n} \sum_{j=i}^{n} (\beta_i - \gamma_i)(\beta_j-\gamma_j)
$$
$$ \geq \frac{1}{4fT} \sum_{i,j=1}^{n} (\beta_i - \gamma_i)(\beta_j-\gamma_j) = \frac{1}{4fT} \left( \sum_{i=1}^{n} (\beta_i - \gamma_i)\right)^2. $$
Finally, we use the fact that $\sum_{i=1}^{n} (\beta_i - \gamma_i) = \EX[\sum_{i=1}^{n} (X_i-T)_+ -  (X_i-(1+f)T)_+] \geq \EX[(X_{\max} - T)_+ - (X_{\max} - (1+f)T)_+] = (\beta - \gamma) \EX[X_{\max}]$ (since all the terms in the sum are positive, and $X_{\max}$ must be one of them). Also, from above, $\EX[X_{\max}] \geq  \frac{T}{2(1-\beta)}$. To summarize, the gain over $\frac12 \EX[X_{\max}]$ is
$$ \frac12 \sum_{i=1}^{n} \EX[(X_i-T)_+] \sum_{j=i}^{n} \Pr[X_j \geq T] \geq 
\frac{1}{4fT} (\beta - \gamma)^2 \EX[X_{\max}]^2  
\geq \frac{(\beta-\gamma)^2}{8 f (1-\beta)} \EX[X_{\max}].
$$

\end{proof}

\subsection{Case 3: high values for buyback}

Finally, we consider the case where $\EX[(X_{\max} - (1+f) T)_+] = \gamma \cdot \EX[X_{\max}]$ is significant. This is actually the only case where we leverage the possibility of buyback, and our analysis only takes advantage of the first buyback event. Obviously, our bounds are not the best possible. However, our intuition is that for large $f$, multiple buybacks are not very useful.
We prove the following.

\begin{lemma}
\label{lemma:case3}
Suppose $T = \med(X_{\max})$ and $\EX[(X_{\max} - (1+f)T)_+] = \gamma \cdot \EX[X_{\max}]$.
Then the algorithm with $T$ as a threshold (and 1 possible buyback) achieves
$$ \EX[ALG] \geq \left( \frac{1}{2} + \frac{\ln 2}{2(1+f)} \cdot \gamma \right) \ \EX[X_{\max}].$$
\end{lemma}

\begin{proof}
We use Lemma~\ref{lemma:buyback-bound} in a restricted form, which is that we only count the contributions where $S'=0$ or $S'=1$ in Lemma~\ref{lemma:buyback-bound}. This gives
\begin{eqnarray*}
\EX[ALG] & \geq & T \cdot \Pr[X_{\max} \geq T] + \EX[(X_{\max} - T)_+ \indic(S'=0)] + \EX\left[ \left( \frac{X_{\max}}{1+f} - T \right)_+ \indic(S'=1) \right] \\
& = & T \cdot \Pr[X_{\max} \geq T] + \EX[(X_{\max} - T)_+] \cdot \Pr[S'=0] + \EX\left[ \left( \frac{X_{\max}}{1+f} - T \right)_+ \right] \cdot \Pr[S'=1]
\end{eqnarray*} 
where $S' = \sum_{j=1}^{n} \indic(X'_j \geq T)$ and $X'_1,\ldots,X'_n$ are independent copies of $X_1,\ldots,X_n$. 

We have $\Pr[S'=0] = \Pr[\forall j; X'_j < T] = \Pr[X_{\max} < T] = 1/2$, and we use Lemma~\ref{lemma:Poisson-compare} to bound the probability that $S'=1$.
 By Lemma~\ref{lemma:Poisson-compare}, $S'$ is stochastically dominated by a Poisson variable with mean $\lambda = \ln 2$, and 
$$ \Pr[S' \leq 1] \geq e^{-\lambda} + \lambda e^{-\lambda}.$$
We have $\Pr[S'=0] = \frac12= e^{-\lambda}$, and so $\Pr[S'=1] \geq \lambda e^{-\lambda} = \frac{\ln 2}{2}$. Thus, we obtain
\begin{eqnarray*}
\EX[ALG] & \geq & \frac12 T + \frac12 \EX[(X_{\max} - T)_+] + \frac{\ln 2}{2} \EX\left[ \left( \frac{X_{\max}}{1+f} - T \right)_+ \right] \\
& \geq & \frac12 \EX[X_{\max}] + \frac{\ln 2}{2(1+f)} \cdot \gamma \cdot \EX[X_{\max}].
\end{eqnarray*}
\end{proof}

\subsection{Combining the cases}

\begin{corollary}
There is an order oblivious algorithm for the prophet inequality with buyback factor $f$ which achieves 
$$ \EX[ALG] \geq \left(\frac12 + \frac{1}{50(1+f)} \right) \EX[X_{\max}].$$
\end{corollary}

\begin{proof}
If $f < 0.37$, then Theorem~\ref{thm:small-factor} gives the desired bound.

If $f\geq 0.37$ and $\beta < 0.39$, Lemma~\ref{lemma:case1} gives a factor at least $\frac{4-0.39}{7} > \frac12 + \frac{1}{50(1+f)}$.

If $\beta \geq 0.39$ and $\gamma \leq 0.06$, Lemma~\ref{lemma:case2} gives a factor at least $\frac12+ \frac{(0.39-0.06)^2}{8 \cdot 0.31 (1+f)} > \frac12 + \frac{1}{50(1+f)}$.

If $\gamma > 0.06$, Lemma~\ref{lemma:case3} gives a factor at least $\frac12 + \frac{\ln 2}{2(1+f)}\cdot 0.06 > \frac12+ \frac{1}{50(1+f)}$.
\end{proof}
