# Supplementary material for: Prophet Inequalities with Cancellation Costs
Source: arXiv:2404.00527 source file (2026-10-12)
Supplement: Supplementary file 3 [file appendix-T2.tex]

\section{The setting with two random variables}
\label{apx:optimal-two}
In this section we prove the optimal online algorithm can get $\frac{1+f}{1+2f} \EX[X_{\max}]$ when there are 2 random variables.
\begin{lemma}
    \begin{align*}
        \EX[ALG|X_1 = x_1] \geq \frac{1+f}{1+2f} \EX[X_{\max}|X_1 = x_1]
    \end{align*}
\end{lemma}
\begin{proof}
    \begin{align*}
        \EX[ALG|X_1 = x_1] &= \max \left(\EX[X_{2}], x_1 + \EX[(X_{2}-(1+f)x_1)_+]\right)\\
        & \geq \frac{f}{1+2f}\EX[X_{2}] + \frac{1+f}{1+2f} \left(x_1 + \EX[(X_{2}-(1+f)x_1)_+]\right) \\
        & = \frac{1+f}{1+2f}\left(x_1 + \EX\left[\frac{f}{1+f}X_{2}+(X_{2}-(1+f)x_1)_+\right] \right)\\
        & \geq \frac{1+f}{1+2f}\left( x_1 + \EX[(X_{2}-x_1)_+] \right) \\
        & = \frac{1+f}{1+2f}\EX[X_{\max}|X_1 = x_1]
    \end{align*}
    The first inequality comes from the fact that $\max$ is always greater than any convex combination and the second inequality holds point-wise for any realization of $X_2$.
\end{proof}
\noindent In order to finish the proof notice that:
\begin{align*}
    \frac{\EX[ALG]}{\EX[X_{\max}]} = \frac{\EX[\EX[ALG|X_1 = x_1]]}{\EX[\EX[X_{\max}|X_1 = x_1]]} \geq \min_{x_1}\frac{\EX[ALG|X_1 = x_1]}{\EX[X_{\max}|X_1 = x_1]} \geq \frac{1+f}{1+2f}.
\end{align*}
